# Supplementary material for: Band-filling-controlled magnetism from transition metal intercalation in $N_{1/3}$NbS$_2$ revealed with first-principles calculations
Source: arXiv:2305.08743 source file (2023-05-15)
Supplement: Supplementary file 1 [file sm.pdf]

# Supplemental material for "Band-filling-controlled magnetism from transition metal intercalation in $N_{1/3}NbS_2$ revealed with first-principles calculations"

Z. Hawkhead,[1] T. J. Hicken,[1,2] N. P. Bentley,[1] B. M. Huddart,[1,3] S. J. Clark,[1] and T. Lancaster[1]

[1]*Department of Physics, Centre for Materials Physics, Durham University, Durham, DH1 3LE, United Kingdom*
[2]*Department of Physics, Royal Holloway, University of London, Egham, TW20 0EX, United Kingdom*
[3]*Oxford University Department of Physics, Clarendon Laboratory, Parks Road, Oxford OX1 3PU, United Kingdom*

In this Supplemental Material we present additional computational details that would allow one to reproduce our work, as well as further justification for some of the choices made in this work. We present additional comparison between the spin-only magnetic moment and experimental measurements, as well as densities of states that show the same results as presented in the main text in a different format. We also provide a complete set of Fermi surfaces.

## ADDITIONAL COMPUTATIONAL DETAILS

The calculations carried out in this work are detailed in the main text. When performing the calculations, for each material a plane-wave cut off of 1700 eV was used along with a Monkhorst-Pack $\boldsymbol{k}$-point grid of 7×7×7 for convergence better than 1 meV/atom. Exchange and correlation was treated using the PBE functional [? ]. Each calculation was performed using the density mixing scheme. We use ultra-soft pseudopotentials throughout. In the main text we discuss the inclusion of a Hubbard $U$ in the calculations. A Hubbard $U$ acts as a local Coulombic repulsion which is often used to address the band gap problem, but in magnetic ions it can be used to localise spin.

Measurements of the lattice constants of materials in this series demonstrate that they change little upon intercalation, with the $a$ lattice parameter changing by less than 1%, while the $c$ lattice parameter changes by up to 6% [? ? ? ]. The relatively small changes in the lattices are due to the weak van der Waals forces acting between the $NbS_2$ layers. As van der Waals forces are not captured by the PBE functional, it is impractical to perform geometry optimisation on this type of quasi two-dimensional materials, since they often result in the layers drifting unphysically far apart. The lattice parameters of each material were therefore held fixed at the experimental values of $Co_{1/3}NbS_2$, $a = b = 5.77$ Å, $c = 11.89$ Å. Holding these parameters fixed across the series has little effect on the residual forces calculated in the materials. In each case the $N$ and Nb ions experience no resultant force while the force on the S ions is typically much less than 1 eV/Å and uncorrelated with the size of intercalated ion.

To extract the orbital population and spin on each atom that is shown in the main text, we use a Mulliken projection. For $N_{1/3}NbS_2$ ($N$ = Ti, V, Mn, Fe, Co, Ni), we find that Mulliken projection is an excellent method for describing orbital populations with spilling parameters less than 0.5% for each material, showing that the electron density can be well represented by an atomic orbital description. Calculation of the band structure in these materials at the specified precision is relatively inexpensive, averaging around 45 CPU hours per material.

| | DFT | | | | Experimental |
|---|---|---|---|---|---|
| $M$ | $n_\uparrow$ | $n_\downarrow$ | $n_\uparrow - n_\downarrow$ | $\mu_s$ ($\mu_B$) | $\mu_{exp}$ ($\mu_B$) |
| Ti | 6.37 | 5.15 | 1.22 | 1.98 | 1.76 |
| V | 7.55 | 5.05 | 2.50 | 3.35 | 2.93(3) |
| Cr | 8.63 | 5.12 | 3.51 | 4.40 | 3.6(2) |
| Mn | 9.47 | 5.17 | 4.30 | 5.20 | 5.1(2) |
| Fe | 5.42 | 2.21 | 3.21 | 4.09 | 4.8(2) |
| Co | 5.32 | 3.47 | 1.85 | 2.67 | 3.0(5) |
| Ni | 5.40 | 4.47 | 0.94 | 1.66 | 2.4(3) |

TABLE S1. The magnetic moment of $N_{1/3}NbS_2$. Calculations are performed directly using the results of the density functional theory calculations. $n_{\uparrow,\downarrow}$ is the number of spin up or down electrons respectively on the $N$ atom that are included in the ultrasoft psuedopotential, such that the spin-only moment $\mu_s = \sqrt{(n_\uparrow - n_\downarrow)[(n_\uparrow - n_\downarrow) + 2]}$. Experimental moments are an average (with a standard error when more than one value is available) of data from Refs. [? ? ? ? ? ? ? ? ? ? ? ? ].

## MAGNETIC MOMENTS

In a collinear spin-DFT calculation, an artifical spin-quantisation axis is imposed on the electrons, typically along the $z$-axis. Using Mulliken projection allows for a good approximation for the spin along the $z$-axis for a particular atom or ion, however this is generally not what is measured experimentally. In Tab. ?? we show equivalent computations of the spin-only moment as in the main text, using instead the values obtained by Mulliken analysis. The number of electrons shown are the ones included in the pseudopotential for each species. Using the results of the DFT, we again find good agreement with experiment.

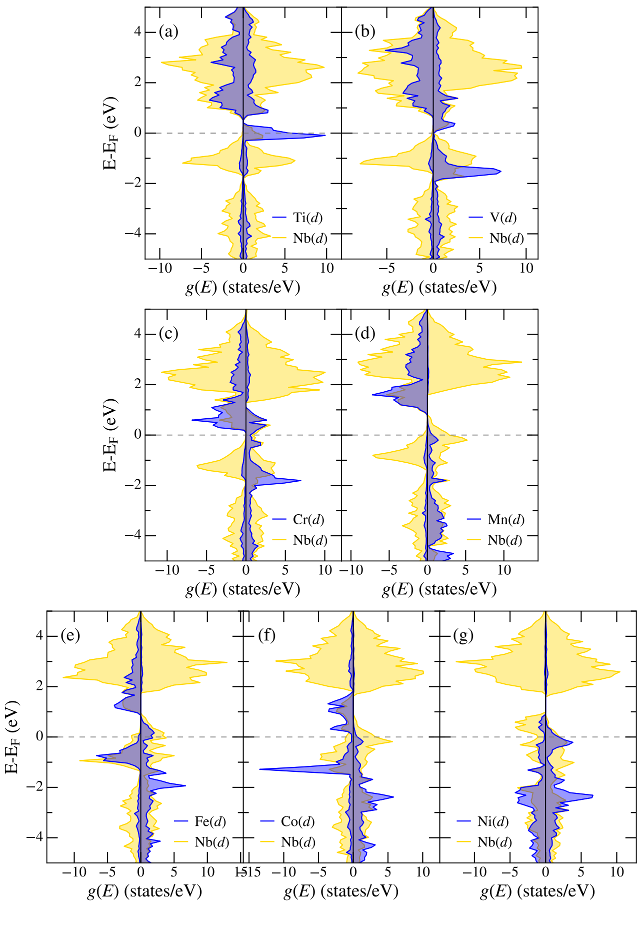

FIG. S1. Partial densities of states of $N_{1/3}NbS_2$ ($N$ = Ti, V, Cr, Mn, Fe, Co, Ni) showing the contribution for the $d$-orbitals in the transition metals. Spin-up and spin-down densities are shown as positive and negative respectively.

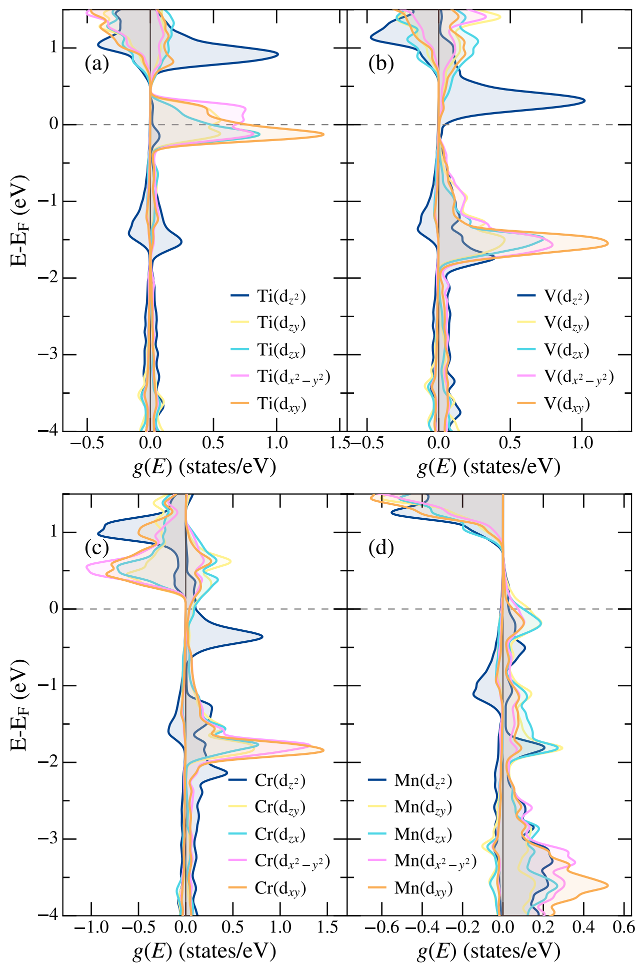

FIG. S2. Projected density of states of the $3d$ orbitals of the intercalate ions in the first half of the period. One can see that the contribution to the DoS from the intercalant $3d_{z^2}$ orbital is lower in energy than the other orbitals.

## DENSITY OF STATES

We present calculations of the DoS of $N_{1/3}NbS_2$ ($N$ = Ti, V, Cr, Mn, Fe, Co, Ni). The DoS around the Fermi energy is dominated by contributions from the $N$ $3d$ electrons and the Nb $4d$ electrons. We therefore show the partial DoS for these electrons in Fig. ??. The DoS have been generated from the electronic structure calculations by applying the adaptive broadening technique described by ? ]. On the left-hand-side of Fig. ?? we see that the shape and position of the spin-down channels are qualitatively the same for $N$ = Ti, V, and Mn, which mirrors the observations of the band structures shown in the main text. We can identify a peak in the spin-up channel in these materials, firstly for $N$ = Ti, which lies at the Fermi energy ($E_F$). As we progress through the series to $N$ = Cr, this peak moves down (equivalently, $E_F$ increases). In the case of $N$ = Mn, this peak is less clear. For the materials on the other end of the series, we see analogous results in the spin-down DoS. We identify a different peak in $N$ = Fe, which can be seen at decreasing energies in $N$ = Co and Ni. This effect is shown quantitatively in the main text. In many of the materials we can also identify a region of reduced DoS in the spin-down channel that we previously saw in $Cr_{1/3}NbS_2$ [? ], allowing the identification of $Cr_{1/3}NbS_2$ as a half-metal. However, only for the materials where the intercalant $3d$-orbital is less than half-filled, such as $Cr_{1/3}NbS_2$, do we find this reduction at the Fermi level. In $Cr_{1/3}NbS_2$, we found that a small reduction in the DoS in the spin-up channel, termed a pseudogap, is responsible for low-temperature fluctuations in the magnetism, and consequently, for the low-temperature magnetic and transport properties [? ].

Figure ?? shows the contribution to the DoS from the individual $3d$ orbitals of the intercalant for the materials formed by intercalating $NbS_2$ with elements from the first half of the first period. We see that there is a significant peak in the DoS from the $d_{z^2}$ orbital sitting below

$E_F$ in both the spin-up and spin-down channels. This is consistent with the energy splitting expected due to the local symmetry environment of the intercalate, as discussed in the main text. The broken degeneracy of the $d$ orbitals allows for an explanation of the differences between the calculated electron filling mechanism and the observed filling of the independent atom. The $d_{z^2}$ orbital is sufficiently low in energy that the energy cost of having this orbital doubly occupied is outweighed by the energy savings of filling a lower energy state.

## FERMI SURFACES

We calculated Fermi surfaces in $N_{1/3}NbS_2$ ($N$ = Ti, V, Cr, Mn, Fe, Co, Ni) by taking the energy of the bands as a function of $\boldsymbol{k}$-space and finding which bands cross the Fermi energy. From these bands, we then calculate the position in $\boldsymbol{k}$-space where these bands cross the Fermi energy, resulting in a number of surfaces. We show the Fermi surfaces for the materials not presented in the main text in Fig. **??**. It is possible to identify Fermi surface nesting in the second half of the period, as well as for $N$ = Mn which is an intermediate case. For example, in $N$ = Ni we see almost cylindrical surface for the spin-up electrons. This nesting could suggest the ability to form spin-density waves which would lead to the ferromagnetic configuration considered in these calculations being unstable, resulting in an antiferromagnetic exchange interaction. The experimentally observed groundstate of $Ni_{1/3}NbS_2$ is indeed antiferromagnetic.

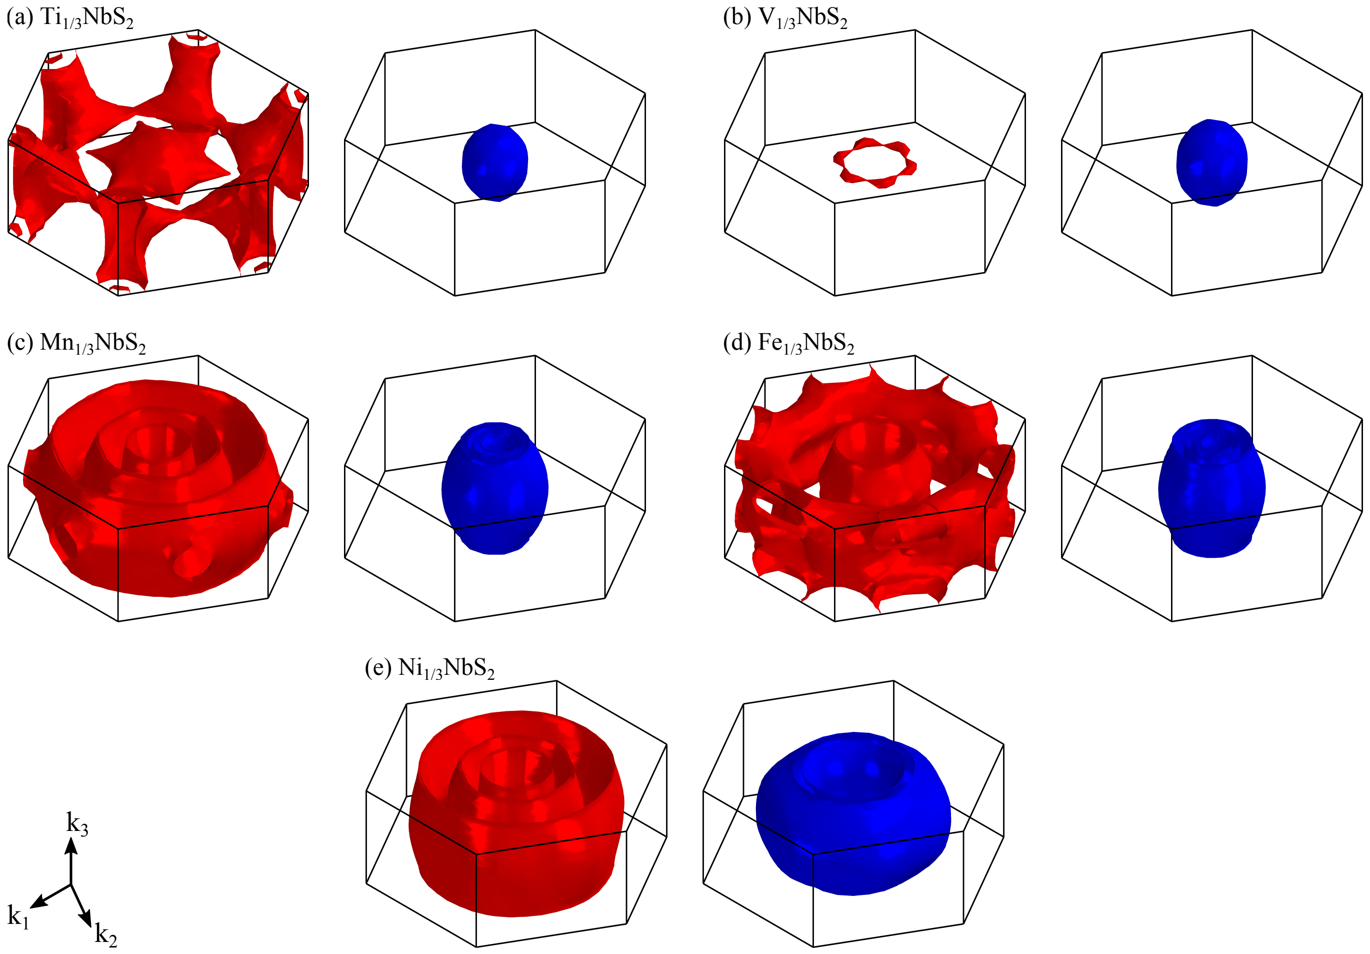


FIG. S3. Fermi surfaces of $N_{1/3}NbS_2$ ($N$ = Ti, V, Mn, Fe, Ni) with the Fermi surfaces of the spin-up and spin-down electrons shown in red and blue respectively.
